# Supplementary material for: Unsupervised Few-Shot Action Recognition via Action-Appearance Aligned Meta-Adaptation
Source: arXiv:2109.15317 source file (2021-10-11)
Supplement: Supplementary file 1 [file dataset_ablation.tex]

\begin{table*}[ht]
\centering
\resizebox{\textwidth}{!}{%
\begin{tabular}{c|c|c|c|c|c|c|c|c|c|c|c|c|}
\cline{2-13}
 & \multicolumn{4}{c|}{UCF101 (unlabeled)} & \multicolumn{4}{c|}{HMDB51 (unlabeled)} & \multicolumn{4}{c|}{Kinetics100 (unlabeled)} \\ \cline{2-13} 
 & \multicolumn{2}{c|}{Base Class} & \multicolumn{2}{c|}{$+$ large unlabeled} & \multicolumn{2}{c|}{Base Class} & \multicolumn{2}{c|}{$+$ large unlabeled} & \multicolumn{2}{c|}{Base Class} & \multicolumn{2}{c|}{$+$ large unlabeled} \\ \hline
\multicolumn{1}{|c|}{Methods} & 1-shot & 5-shot & 1-shot & 5-shot & 1-shot & 5-shot & 1-shot & 5-shot & 1-shot & 5-shot & 1-shot & 5-shot \\ \hline
\multicolumn{1}{|c|}{CVRL \cite{qian2020spatiotemporal}} & 53.46 $\pm$ 0.46 & 75.41  $\pm$  0.40 & 63.00  $\pm$  0.41 & 87.80  $\pm$  0.30  & 27.45 $\pm$ 0.38  & 30.91  $\pm$ 0.36 & 44.21  $\pm$  0.45 & 60.35  $\pm$  0.45 & 43.00  $\pm$ 0.41 & 58.35  $\pm$  0.43 & 53.26  $\pm$  0.48 & 71.39  $\pm$  0.44 \\ \hline
\multicolumn{1}{|c|}{\methodname~(Ours)} & 65.31 $\pm$ 0.39  & 85.26 $\pm$ 0.47  & \textbf{76.38 $\pm$ 0.40} & \textbf{92.50 $\pm$ 0.24} & 36.72 $\pm$ 0.34 & 51.43 $\pm$ 0.45  & \textbf{47.55 $\pm$ 0.45}  &  \textbf{66.13 $\pm$ 0.33} & 50.28 $\pm$ 0.47 & 65.92 $\pm$ 0.44  & \textbf{62.80 $\pm$ 0.45} & \textbf{79.55 $\pm$ 0.39} \\ \hline
\end{tabular}%
}
\caption{\textbf{Efficacy of acquiring and training on large unlabeled video dataset}. We compare the 1 and 5 shot 5-way performance of training models individually on `Base Class' videos and in addition with the `large-unlabeled' video dataset (total $\sim$550K videos). We compare our method against CVRL~\cite{qian2020spatiotemporal} which is the best-performing unsupervised baseline method. Unsupervised training on large-scale unlabeled dataset outperforms training on just base class video by a significant margin. For both data scenarios, \methodname~also significantly outperforms state-of-the-art CVRL that highlights the significance of having action-appearance aligned representations and an explicit few-shot learner to meta-learn from unlabeled videos.}

% \textbf{76.38 $\pm$ 0.40}  & \textbf{92.50 $\pm$ 0.24} & \textbf{47.55 $\pm$ 0.45}  &  \textbf{66.13 $\pm$ 0.33} & \textbf{62.80 $\pm$ 0.45} & \textbf{79.55 $\pm$ 0.39}
\label{tab:data_ablation}
\end{table*}
