# Supplementary material for: Unsupervised Few-Shot Action Recognition via Action-Appearance Aligned Meta-Adaptation
Source: arXiv:2109.15317 source file (2021-10-11)
Supplement: Supplementary file 2 [file backbone_ablation.tex]

\begin{table*}[t]
\centering
\resizebox{0.8\textwidth}{!}{%

\begin{tabular}{|l|r|c|c|c|c|c|c|}
\hline
\multirow{2}{*}{3D Action Encoder} & \multirow{2}{*}{Params} & \multicolumn{2}{c|}{UCF101} & \multicolumn{2}{c|}{HMDB51} & \multicolumn{2}{c|}{Kinetics100} \\ \cline{3-8} 
  & & 1-shot & 5-shot & 1-shot & 5-shot & 1-shot & 5-shot \\ \hline

S3D~\cite{xie2018rethinking}  & 9.6M & 66.09 $\pm$ 0.46 & 88.42 $\pm$ 0.31 & 40.92 $\pm$ 0.47   & 61.03 $\pm$ 0.46  & 54.83 $\pm$ 0.48 & 73.64 $\pm$ 0.42 \\ 
C3D~\cite{tran2015learning}   & 27.7M &  72.00 $\pm$ 0.42 & 90.88 $\pm$ 0.27 & 43.51 $\pm$ 0.47 & 63.70 $\pm$ 0.46 & 58.52 $\pm$ 0.46 & 76.93 $\pm$ 0.40 \\ 
 R(2$+$1)D-34~\cite{tran2018closer}   & 64.0M &  67.06 $\pm$ 0.45 & 89.06 $\pm$ 0.30 & 41.51 $\pm$ 0.46 & 61.72 $\pm$ 0.46 & 55.63 $\pm$ 0.47 & 74.09 $\pm$ 0.42 \\ 
Resnet50-3D~(Ours) & 44.5M &  \textbf{76.38 $\pm$ 0.40}  & \textbf{92.50 $\pm$ 0.24} & \textbf{47.55 $\pm$ 0.45}  &  \textbf{66.13 $\pm$ 0.33} & \textbf{62.80 $\pm$ 0.45} & \textbf{79.55 $\pm$ 0.39} \\ 
\hline
\end{tabular}%
}
\caption{Ablation study of \methodname~highlighting the choice of using ResNet-3D-50 as the 3D Action encoder compared to contemporary 3D architecture designs used by previous methods. ResNet-3D-50 is able to outperform all other backbones across all few-shot benchmarks.}
\label{tab:backbone_ablation}

\end{table*}
